# Supplementary material for: Forest Floor Visualizations of Random Forests
Source: arXiv:1605.09196 ancillary file (2016-07-04)
Supplement: Supplementary file 1 [file 1605.09196_suppl.mat.pdf]

This document is the supplementary materials for article "Forest Floor Visualizations of Random Forests" <http://arxiv.org/abs/1605.09196v1>

# Supplementary materials for: ”*Forest Floor Visualizations of Random Forests*”.

Soeren H. Welling, Line K.H. Clemmensen, Hanne H.F. Refsgaard, & Per B. Brockhoff

May 31, 2016

## 1 Proof for Equation [11] and [12] of article.

**Part 1 - Any sequence of  $d$ -dimensional vectors:** Denote a sequence of  $n+1$  real vectors (or scalars) describing points in a  $\mathbb{R}^d$   $d$ -dimensional space as  $\hat{y}''_k$  for  $k \in \{0, \dots, n\}$ . The difference between any two adjacent vectors is defined as  $L_k = \hat{y}''_k - \hat{y}''_{k-1}$  for  $k \in \{1, \dots, n\}$ .

**Lemma 1:**

$$\hat{y}''_n = \sum_{k=1}^n L_k + \hat{y}''_0 \quad (1)$$

**Proof 1:**

For  $k \in \{1, \dots, n\}$ ,  $\hat{y}''_k$  is the additive part of  $L_k$  and  $\hat{y}''_{k-1}$  the subtractive part.

When summing every  $L_k$ , all intermediary vectors of the sequence cancel out.

$$\sum_{k=1}^n L_k = (\hat{y}''_1 - \hat{y}''_0) + (\hat{y}''_2 - \hat{y}''_1) + (\hat{y}''_n - \hat{y}''_{n-1}) = \hat{y}''_n - \hat{y}''_0$$

Replacing  $\sum_{k=1}^n L_k$  with  $\hat{y}''_n - \hat{y}''_0$  in stated Lemma 1, one obtain

$$\hat{y}''_n = \hat{y}''_n - \hat{y}''_0 + \hat{y}''_0$$

**Part 2 - a single tree:** A tree is a hirachial graph. The first node, node 0, is connected to node 1. Every node from node 1 is either terminal and only connected to one parent node or

an intermediary node and has two daughter nodes. Every node of a tree has a prediction  $\hat{y}_k''$  which is a real vector/scalar with exactly  $d$  dimensions.

## Notes for part 2

*For regression, a node prediction is a real scalar and computed as the target mean of inbag samples passing through the node. For classification a vector of  $d$  dimensions, where  $d$  is the number of classes in the training set, and each element from 1 to  $d$  describe the prevalence ratio of inbag samples by a given class. Notice some random forest implementation use majority voting in terminal nodes. Here majority class element will be 1 and the remaining 0. Virtually any other prediction rule for nodes in classification trees outputting real valued vectors of length  $|\hat{y}_k''|^1 = 1$  would be acceptable. Virtually any other prediction rule for nodes in regression trees outputting real values would be acceptable.*

An observation is an entity which will take one direct path of steps through the tree, starting from node 0 and ending in a terminal node. Observations are enumerated for  $i \in \{1, \dots, N\}$ . Each observation will attain a sequence of predictions, one for each node it passes through. Each prediction is a real vector/scalar and written  $\hat{y}_{ik}''$ , where  $k$  sequentially enumerates the  $n$  nodes of the path for observation  $i$ . As  $n$  may differ for each observation  $i$ , it is thus written  $n_i$ . In one tree, any observation step sequence share the same first node 0 and node 1 also called the root node of the tree. A local increment ( $L_{ik}$ ) is defined as a vector describing the prediction difference from  $(k-1)^{th}$  to the  $k^{th}$  node for observation  $i$ .

Therefore we write  $L_{ik} = \hat{y}_{i,k}'' - \hat{y}_{i,k-1}''$  for  $k \in \{1, \dots, n\}$  for  $n_i \geq 1$ .

The first node  $y_0$  of one tree contain all observations and the prediction is the training set base rate / grand mean.  $y_0$  can also be written as  $\bar{y}$ . The tree prediction of the  $i^{th}$  observation  $\hat{y}_i'$ , is defined as defined as the terminal node  $\hat{y}_i' = \hat{y}_{ik}''$  where  $k = n_i$ .

## Lemma 2

$$\hat{y}_i' = \sum_{k=1}^{n_i} L_{ik} + \bar{y} \text{ for any } i \in \{1, \dots, N\} \quad (2)$$

**Proof 2:** As a given sequence of node predictions  $\hat{y}_{ik}''$  for a given observation  $i$  are real

vectors/scalars, then the local increments of this sequence must be a part of any sequence postulated in lemma 1. Replacing  $\bar{y}$  with  $y_0$  and  $\hat{y}'_i$  with  $\hat{y}''_n$  we obtain lemma 1. Thus lemma 2 must be true also.

**Part 3 - the test set prediction of any ensemble of trees** The tree prediction of the  $i^{th}$  observation of the  $j^{th}$  tree is written  $\hat{y}'_{ij}$ . An ensemble prediction  $\hat{y}_i$  of  $ntree$  decision trees is equal to the mean of the tree predictions  $\hat{y}'_{ij}$  for each  $i$  observation.  $\hat{y}_i = \frac{1}{ntree} \sum_j^{ntree} \hat{y}'_{ij}$  for A local increment of the  $j^{th}$  tree  $L_{ik}$  can be written  $L_{ijk}$  the number of local increments/steps for the  $i^{th}$  sample in the  $j^{th}$  tree can be written  $n_{ij}$ .

**Lemma 3**

$$\hat{y}_i = \frac{\sum_{j=1}^{ntree} \sum_{k=1}^{n_{ij}} L_{ijk}}{ntree} + \bar{y}, \quad (3)$$

**Proof 3:**

$$\begin{aligned} \hat{y}_i &= \frac{\sum_{j=1}^{ntree} \sum_{k=1}^{n_{ij}} L_{ijk}}{ntree} + \bar{y} \\ \hat{y}_i &= \frac{\sum_{j=1}^{ntree} \sum_{k=1}^{n_{ij}} (L_{ijk} + \bar{y})}{ntree}, \text{ use Lemma 2 to replace } L_{ijk} \text{ with prediction of } j^{th} \text{ tree } \hat{y}'_{ij} \\ \hat{y}_i &= \frac{\sum_{j=1}^{ntree} \hat{y}'_{ij}}{ntree}, \text{ this is the definition of the ensemble prediction} \end{aligned}$$

**Part 4** For any  $j^{th}$  tree, any training observation  $i$  is either be designated as inbag or out-of-bag (OOB). The OOB prediction  $\tilde{y}_i$  computed from a subset of all trees  $\{1, \dots, ntree\}$  where  $i$  is OOB, we call this subset for  $\tilde{J}_i$  and this set will have  $nOOB_{tree,i}$  members. The OOB ensemble prediction is defined as the mean prediction of OOB tree for the  $i^{th}$  observation.  $\tilde{y}_i = \frac{1}{nOOB_{tree,i}} \sum_{j \in \tilde{J}_i} y_{ij}$  where subset  $\tilde{J}_i \subseteq \{1, \dots, ntree\}$ .

**Lemma 4**

$$\tilde{y}_i = \frac{\sum_{j \in \tilde{J}_i} \sum_{k=1}^{n_{ij}} L_{ijk}}{ntree} + \bar{y} \quad (4)$$

Proof 4: As lemma 3 was shown for any set of trees in an ensemble, and as lemma 4 is just the special case for particular subsets of trees, then lemma 4 must be true also.

## 1.1 How to highlight the mapping structure of a local cluster

In the white wines quality (wwq) data set. A local interaction was identified among wines with the lowest alcohol content ( $< 9.3\%$ ). In spite of low alcohol content in general lead to lower preference predictions, a subgroup of low alcohol wines deviated from this main effect. It was possible to further characterize this local interaction in the mapping structure of the trained RF model. Any wine of alcohol content more than 9.3 was colored transparent grey. Remaining low alcohol wines were colored by the feature contribution of alcohol, such that wines with a relatively positive impact of low alcohol content were marked blue and wines with a relatively negative impact were marked red. Intermediate wines were green. Main effect plots by all features were colored by these scheme as depicted. Hereby it was possible to visualize the local interaction. It was possible to observe that the most clear differences between wines marked blue and wines marked red was the content of chlorides, citric acid and residual sugar. This observation characterized a certain cluster of fruity wines (acidic and sweet) of high preference despite low alcohol content.

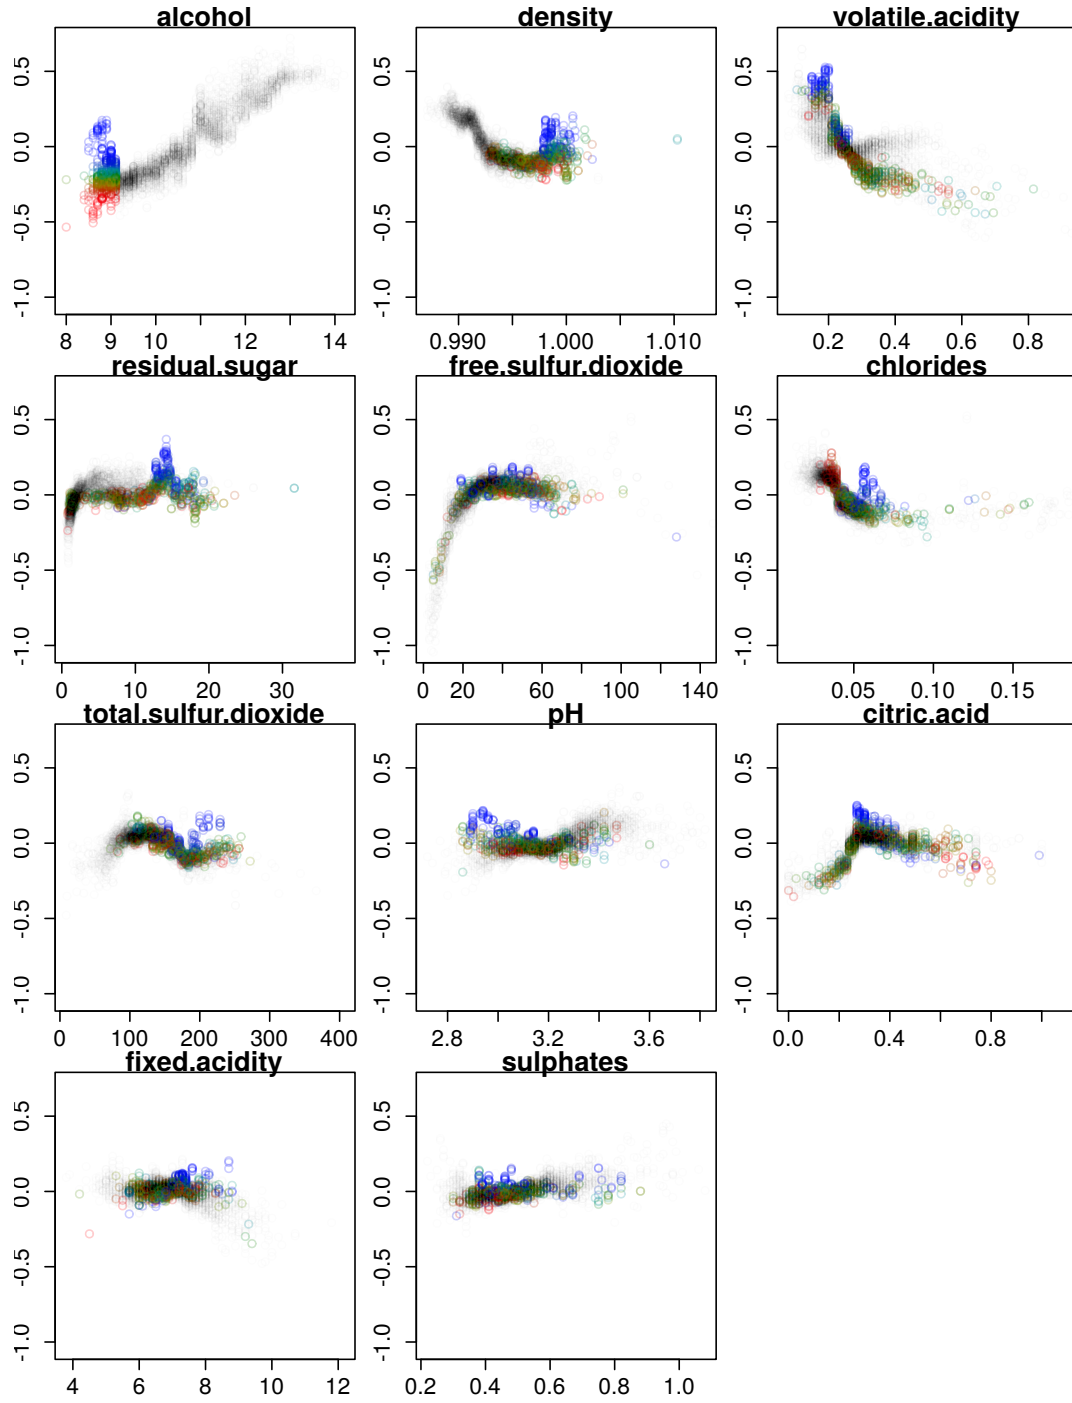

Figure 1: Cross-validated main effect feature contributions of predicted preferences of 4900 white whines. The color gradient along feature contributions of alcohol characterizes the specific interaction pattern between low alcohol content and remaining features.

## 1.2 RF mapping unrelated to data structure

Two normal distributed( $N(0,1)$ ) variables  $x_1$  and  $x_2$  is related to a target  $y$  by either  $G_1(X) = y_1 = (x_1)^2 + 2\sin(2x_2)$  or  $G_2(X) = y_2 = x_1x_2$ . 3000 samples were drawn and a default RF-model was trained. A grid of 300 grid lines and  $300^2$  grid points was formed. Each grid point represented a combination of  $x_1$  and  $x_2$  from  $-7$  to  $7$  such that the entire grid extended the range of sampled values 3 times. Any grid point of  $x_1$  and  $x_2$  was predicted by the RF model. The predicted  $\hat{y}$  was plotted as a function of  $x_1$  and  $x_2$  in a 3D plot. The mapping structure was represented as a surface outlined by the grid points and colored by high  $\hat{y}$  (red/high, green/low). The mapping of the training set is represented by the set blue points on the mapping surface. For the data structure  $G_1$  there is no unstable boundary effect as the partial quadratic function of  $x_1$  and the partial sine function of  $x_2$  do no interact and simply intersect additively in the region of the training set (blue points). The saddle-point structure of  $G_2$  is not the sum of two additive partial functions. In a rectangular boundary of were training set was observed a series of ripples in the mapping structure was observed. Here predictions alternated between high and low values. This boundary mapping structure do not reflect the data structure of  $G_2$ . Likely as RF only performs univariate splits, it can only capture interaction effects by splitting data into sub groups. As these sub group becomes less populated at the boundaries of the data set the fit becomes markedly unstable.

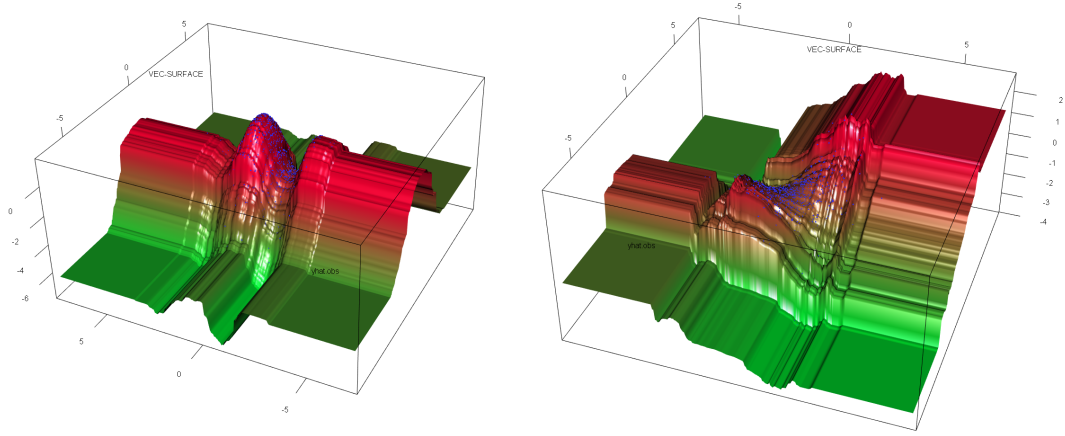

Figure 2: RF regression model structure of two hidden functions  $y_1 = (x_1)^2 + 2\sin(2x_2)$  (left) or  $y_2 = x_1x_2$  (right). Red-green color gradient is parallel to the vertical target axis,  $\hat{y}$ . Positions marked blue are the training examples used to train the mapping structure. The visualized surface extrapolates the training set 100% in each direction. Left plot( $y_1$ ) depicts a stable main effect only structure. Right plot( $y_2$ ) depicts a unstable interaction effect only structure.

### 1.3 Shallowness of Random forest

Although splits of nodes in RF is performed univariately, RF can still capture interactions due to the many local rules applied. Presumably as the sequential decisions performed by RF satisfy only an immediate loss function of each split and splits are only univariate, RF cannot grow decision trees to capture 4<sup>th</sup> order interactions or higher. To test the ability of RF to capture data structures of various complexity, three hidden structures were designed. A series of  $i$  variables  $x_i$  were drawn from a distribution and multiplied. The structure have no error component. Figure 3 depicts from  $d = 1$ (light green) to  $d = 6$ (red) the ability of random forest models to fit a training set of  $N$  train samples. A single main effect is modelled with almost no error already from 100 observations. A second order interaction needs 100-200 samples to explain 75% of the variance when cross validated. A third order interaction in a feature space of continuous variables ("saddle" & "sineprod") requires 10,000 samples to explain 75% variance cross validated.

”saddle”

$$y_d = \prod_{i=1}^d x_i, x_i \in N(0, 1) \quad (5)$$

”sineProd”

$$y_d = \prod_{i=1}^d \sin(x_i), x_i \in U(-\pi/2; \pi/2) \quad (6)$$

”binaryProd” (notice only -1 or 1 is sampled)

$$y_d = \prod_{i=1}^d x_i, x_i \in U\{-1, 1\} \quad (7)$$

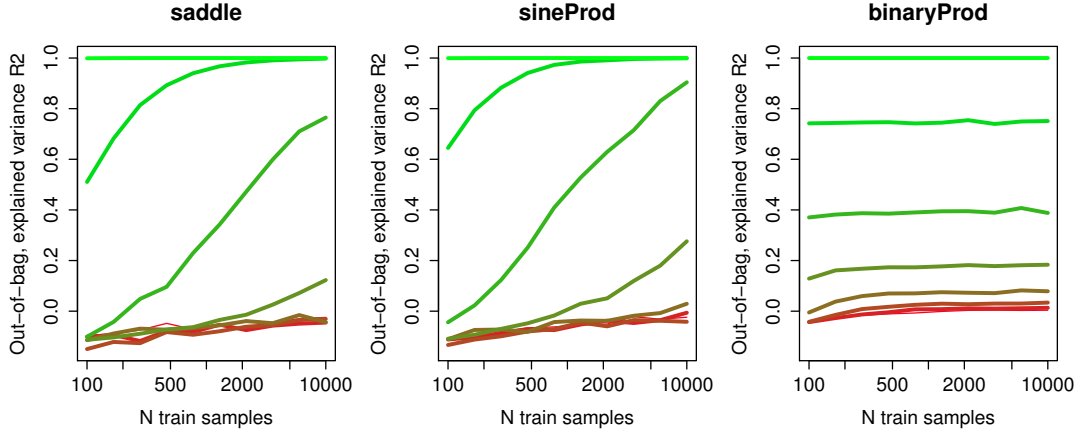

Figure 3: How many orders of interactions can RF capture? Three structures saddle, sineProd and binaryProd, ranging from main effect(light green) 6th order of interaction(red line). RF already becomes an poor estimator at 3rd order interactions.

#### 1.4 The effect of stratification

Stratified bootstrapping by target variable moves weighted centroid of cross validated training predictions to the center of the simplex. Hereby, highly prevalent classes are down-sampled, but every sample will likely participate at least in a small number of trees. Appendix Figure 5 depicts such a stratified RF model, where root node is balanced in respect of target classes. Besides the centroid of prediction were moved to the center of K-1 probability simplex, the general structure of the model structure seemed similar to the non-stratified version in manuscript.

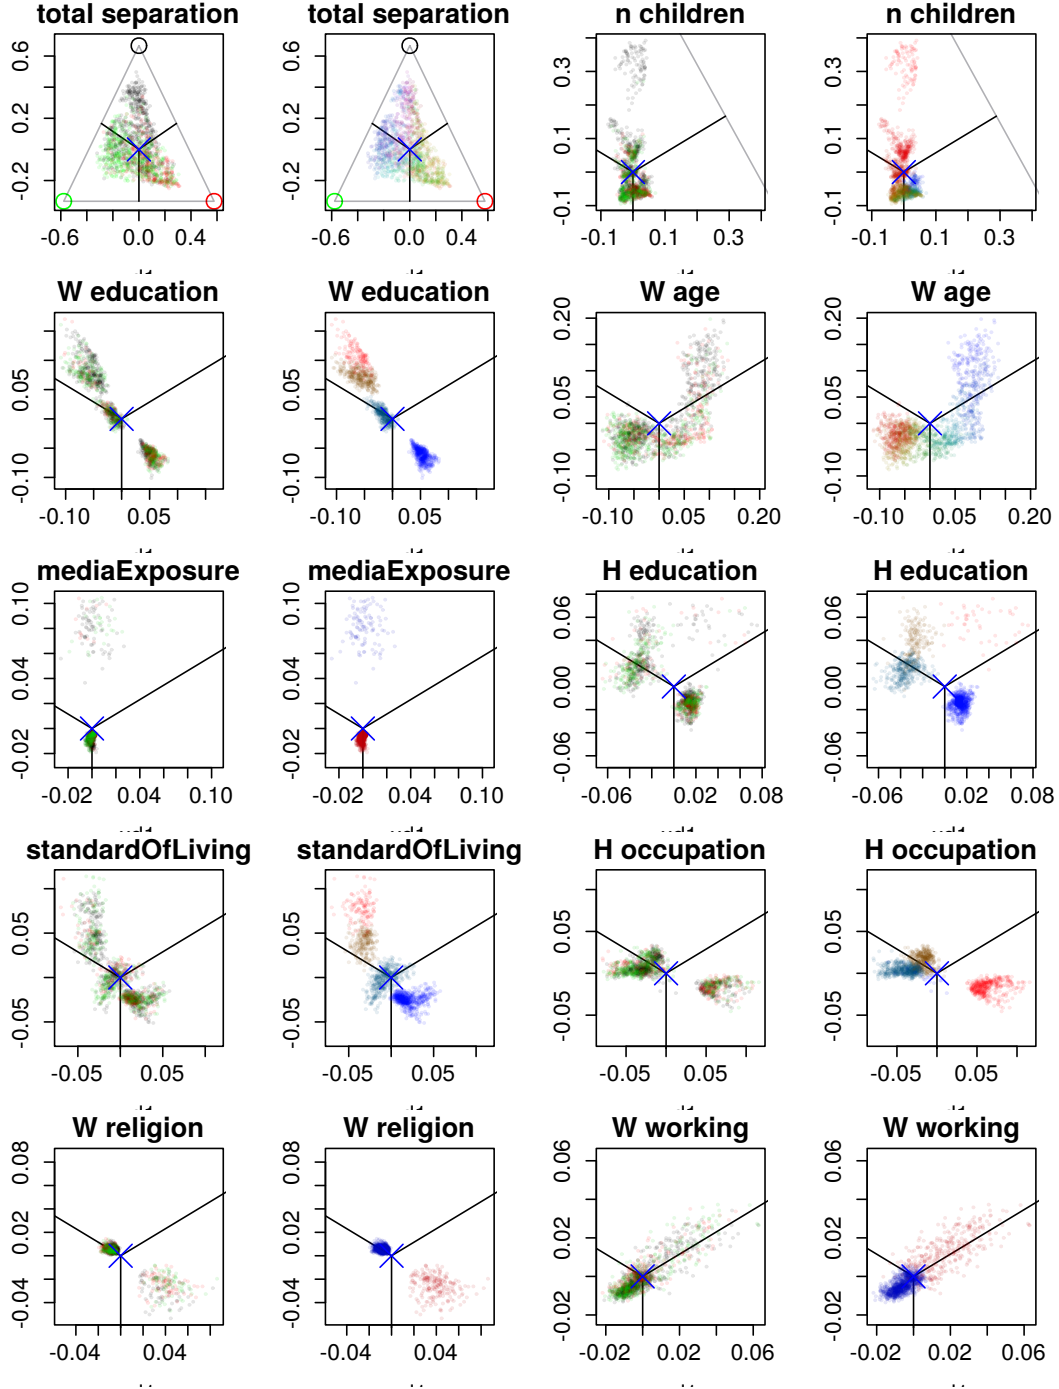

Figure 4: Feature contributions for contraceptive method choice (cmc) data set when RF was trained with target class stratification. Blue cross marks average root node which is also the center of the average cross validated prediction.

## 1.5 forest floor visualizations of gradient boosted tree

Gradient boosted trees suggested by Friedman is a boosted ensemble, where each new tree is fitted to the residuals of the current ensemble of trees [2]. Nonetheless, all grown trees in the ensemble are regular decision trees similar to trees of random forest ensembles. The gradient boosted ensemble prediction is the sum of votes, whereas for a random forest ensemble it is the average vote. In either case, both boosted trees and bagged trees contribute additively to the ensemble prediction. Therefore every prediction can be split into local increments and the feature-wise subtotals, named feature contributions can be computed. Presently, the perhaps most popular gradient boosting algorithm is XGBoost [1]. To make a fast proof-of-concept we preferred not to write an entirely new adaptor for XGBoost, but rather to write a wrapper around the randomForest implementation [3], making it behave as a gradient boosted ensemble and retain compatibility with forestFloor. This short wrapper is printed below and included in the forestFloor package as an example script **ffGradientBoost.R**.

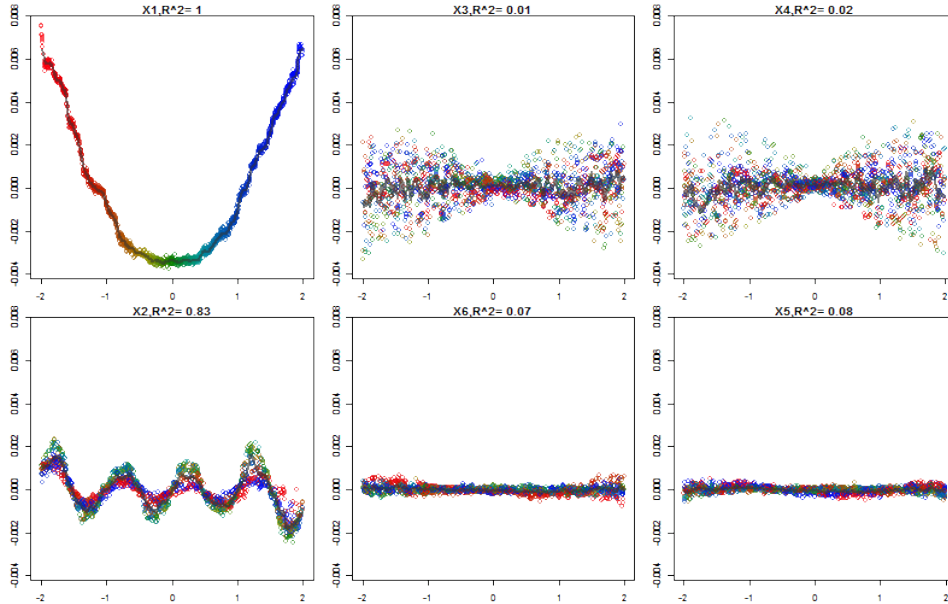

Figure 5: forestFloor visualization of a simpleBoost model. simpleBoost is a gradient boosted tree ensemble, implemented as a simple wrapper of the CRAN randomForest algorithm.

```

1  library(randomForest);library(forestFloor)
3  #simulate data
X      = data.frame(replicate(6,4*(runif(3000)-.5)))
5  Xtest = data.frame(replicate(6,4*(runif(1500)-.5)))
y      = with(X,X1^2+sin(X2*2*pi)+X3*X4) + rnorm(3000)/3
7  ytest = with(Xtest,X1^2+sin(X2*6*pi)+X3*X4) + rnorm(3000)/3

9  #define boosted tree wrapper
simpleBoost = function(
11  X,y,      #training data
    M=100,   #boosting iterations and ntrees
13  v=.1,     #learning rate
    ...) {   #other parameters passed to randomForest
15  y_hat = y * 0 #latest ensemble prediction
    res_hat = 0   #residuals hereof...
17  Fx = list()   #list for trees
    for(m in 1:M) {
19      y_hat = y_hat + res_hat * v #update prediction, by learning rate
        res = y - y_hat             #compute residuals
21      hx = randomForest(X,res,ntree=1,keep.inbag=T,...) #grow tree on residuals
        res_hat = predict(hx,X)      #predict residuals
23      cat("SD=",sd(res), " \n")     #print
        hx$forest$nodepred = hx$forest$nodepred * v #multiply nodepredictions by learning rate
25      Fx[[m]] = hx #append tree to forest
    }
27  Fx = do.call(combine,Fx) #combine trees with randomForest::combine()
    Fx$y = y #append y
29  Fx$oob.times = apply(Fx$inbag,1,function(x) sum(!x)) #update oob.times
    class(Fx) = c("simpleBoost","randomForest") #make simpleBoost a subclass of randomForest
31  return(Fx)
}

33
predict.simpleBoost = function(Fx,X) {
35  class(Fx) = "randomForest"
    predMatrix = predict(Fx,X,predict.all = T)$individual
37  ntrees = dim(predMatrix)[2]
    return(apply(predMatrix,1,sum))
39 }

41 plot.simpleBoost = function(Fx,X,ytest,add=F,...) { #plots learning curve
    class(Fx) = "randomForest"
43  predMatrix = predict(Fx,X,predict.all = T)$individual
    ntrees = dim(predMatrix)[2]
45  allPreds = apply(predMatrix,1,cumsum)
    preds = apply(allPreds,1,function(pred) sd(ytest-pred))
47  if(add) plot=points
    plot(1:ntrees,preds,...)
49  return()
}

```

```

}
51
#build gradient boosted forest
53 rb = simpleBoost(X,y,M=300,replace=F,mtry=6,sampsize=500,v=0.005)

55 #make forestFloor plots
    ffb = forestFloor(rb,X,Xtest)
57 #correct for that tree votes of gradient boosts are summed, not averaged.
    #forestFloor will as default divide by the same number as here multiplied with
59 ffb$FCmatrix = ffb$FCmatrix * c(rb$oob.times,rep(rb$ntree,sum(!ffb$isTrain)))

61 #plot forestFloor for OOB-CV feature contributions and regular feature contributions
    plot(ffb,plotTest=T,col=fcol(ffb,3,plotTest = TRUE))
63 plot(ffb,plotTest=F,col=fcol(ffb,1,plotTest = FALSE))

65 #validate model structure
    pred = predict(rb,X)
67 predtest = predict(rb,Xtest)
    plot(y,pred,col="#00000034")
69 plot(rb,Xtest,ytest,log="x")
    vec.plot(rb,X,i.var=1:2)
71
#export plot
73 png(file = "ffGradientBoost.png", bg = "transparent",width=800,height = 500)
    plot(ffb,plotTest=T,col=fcol(ffb,1))
75 rect(1, 5, 3, 7, col = "white")
    dev.off()

```

## References

- [1] Tianqi Chen and Carlos Guestrin. Xgboost: A scalable tree boosting system. *arXiv preprint arXiv:1603.02754*, 2016.
- [2] Jerome H Friedman. Greedy function approximation: a gradient boosting machine. *Annals of statistics*, pages 1189–1232, 2001.
- [3] Andy Liaw and Matthew Wiener. Classification and regression by randomforest. *R News*, 2(3):18–22, 2002.
